# Supplementary material for: Representing Interlingual Meaning in Lexical Databases
Source: arXiv:2301.09169 source file (2023-01-22)
Supplement: Supplementary file 1 [file APPENDIX.pdf]

## A Appendix: Evaluation Corpus and Method Details

**Lexicalization tables.** Our evaluation corpus is based on the lexicalizations (or the absence thereof) of 32 lexical concepts in nine languages, chosen from five semantic groups known for their cross-lingual diversity (sibling, cousin, rice, watercourse, and horse). Out of  $32 \times 9 = 288$  language-specific word meanings (synsets), 160 are lexicalized and 128 are lexical gaps. The tables below provide the manually assembled lexicalization data from which we produced our evaluation corpus. The left-hand-side columns contain language-independent concepts and their hierarchy, while lexicalizations and their absence (gaps) are shown on the right-hand-side.

| Sibling                 |        |                 |             |                   |      |          |               |                 |             |             |
|-------------------------|--------|-----------------|-------------|-------------------|------|----------|---------------|-----------------|-------------|-------------|
| Meaning                 | Parent | ENG             | FRA         | ITA               | CHI  | HIN      | TAM           | MAL             | HUN         | MON         |
| M0 Sibling              |        | sibling         | GAP         | GAP               | 兄弟姐妹 | सहोदर    | உடன்பிறந்தோர் | കുടുംബപ്പിറപ്പ് | testvér     | GAP         |
| M1 Elder sibling        | M0     | GAP             | ainé        | GAP               | GAP  | GAP      | GAP           | GAP             | nagytestvér | GAP         |
| M2 Younger sibling      | M0     | GAP             | cadet       | GAP               | GAP  | GAP      | GAP           | GAP             | kistestvér  | дүү         |
| M3 Male sibling         | M0     | brother         | frère       | fratello          | 兄弟   | भाई      | சகோதரர்       | സഹോദരൻ          | frútestvér  | GAP         |
| M4 Female sibling       | M0     | sister          | sœur        | sorella           | 姐妹   | बेहेन    | சகோதாரி       | സഹോദരി          | lánytestvér | GAP         |
| M5 Elder male sibling   | M1, M3 | elder brother   | frère aîné  | fratello maggiore | 哥哥   | बड़ा भाई | அண்ணன்        | ചേട്ടൻ          | báty        | ax          |
| M6 Younger male sibling | M2, M3 | younger brother | frère cadet | fratello minore   | 弟弟   | छोटा भाई | தம்பி         | അനിയൻ           | öcs         | эрэгтэй дүү |

| Rice                              |        |            |             |                |     |      |        |        |            |           |
|-----------------------------------|--------|------------|-------------|----------------|-----|------|--------|--------|------------|-----------|
| Meaning                           | Parent | ENG        | FRA         | ITA            | CHI | HIN  | TAM    | MAL    | HUN        | MON       |
| M0 Rice, general term             |        | rice       | riz         | riso           | GAP | GAP  | GAP    | GAP    | rizs       | будаа     |
| M1 Grain still in the husk        | M0     | paddy      | GAP         | risone         | 稻谷  | धान  | நெல்   | നെല്ല് | GAP        | GAP       |
| M2 Uncooked rice, brown or white  | M0     | GAP        | GAP         | GAP            | 米   | चावल | அரிசி  | അരി    | GAP        | GAP       |
| M3 Brown rice, cooked or uncooked | M0     | brown rice | riz complet | riso integrale | GAP | GAP  | GAP    | GAP    | barna rizs | гүц будаа |
| M4 Cooked rice                    | M0     | GAP        | GAP         | GAP            | 米饭  | भात  | சேற்று | ചോറ്   | GAP        | GAP       |
| M5 Uncooked brown rice            | M2, M3 | GAP        | GAP         | GAP            | 糙米  | GAP  | GAP    | GAP    | GAP        | GAP       |
| M6 Uncooked white rice            | M2     | GAP        | GAP         | GAP            | 大米  | GAP  | GAP    | GAP    | GAP        | GAP       |

| Watercourse                      |        |             |             |               |     |        |     |       |           |           |
|----------------------------------|--------|-------------|-------------|---------------|-----|--------|-----|-------|-----------|-----------|
| Meaning                          | Parent | ENG         | FRA         | ITA           | CHI | HIN    | TAM | MAL   | HUN       | MON       |
| M0 Natural body of running water |        | watercourse | cours d'eau | corso d'acqua | 河   | जलधारा | ஓடை | അമ്പല | vízfolyás | урсгал ус |
| M1 Large natural stream of water | M0     | river       | rivière     | fiume         | 川   | नदी    | ஆறு | പുഴ   | follyó    | гол       |
| M2 Very large river              | M0     | GAP         | fleuve      | GAP           | 江   | GAP    | GAP | നദി   | follyam   | мөрөн     |

| Horse                  |        |          |          |          |     |       |             |           |              |        |
|------------------------|--------|----------|----------|----------|-----|-------|-------------|-----------|--------------|--------|
| Meaning                | Parent | ENG      | FRA      | ITA      | CHI | HIN   | TAM         | MAL       | HUN          | MON    |
| M0 Horse, general term |        | horse    | cheval   | cavallo  | 马   | घोड़ा | குதிரை      | കുതിര     | ló           | адуу   |
| M1 Adult horse         | M0     | GAP      | GAP      | GAP      | GAP | GAP   | GAP         | GAP       | GAP          | морь   |
| M2 Young horse         | M0     | foal     | poulain  | puledro  | 小马  | GAP   | GAP         | GAP       | csikó        | унага  |
| M3 Male horse          | M0     | GAP      | GAP      | GAP      | 公马  | घोड़ा | ஆண் குதிரை  | ആൺ കുതിര  | GAP          | хүлэг  |
| M4 Female horse        | M0     | GAP      | GAP      | cavalla  | 母马  | घोड़ी | பெண் குதிரை | പെൺ കുതിര | GAP          | GAP    |
| M5 Male adult horse    | M1, M3 | stallion | étalon   | stallone | GAP | GAP   | GAP         | GAP       | csődör       | азрага |
| M6 Female adult horse  | M1, M4 | mare     | jument   | giumenta | 骡马  | GAP   | GAP         | GAP       | kanca        | гүү    |
| M7 Male young horse    | M2, M3 | colt     | GAP      | GAP      | GAP | GAP   | GAP         | GAP       | csődör csikó | даага  |
| M8 Female young horse  | M2, M4 | filly    | pouliche | puledra  | GAP | GAP   | GAP         | GAP       | kancacsikó   | байдас |

| Cousin                                        |        |          |         |         |     |             |         |        |              |          |
|-----------------------------------------------|--------|----------|---------|---------|-----|-------------|---------|--------|--------------|----------|
| Meaning                                       | Parent | ENG      | FRA     | ITA     | CHI | HIN         | TAM     | MAL    | HUN          | MON      |
| M0 Person related through family relationship |        | relative | parent  | parente | 亲戚  | रिश्तेदार   | உறவினர் | ബന്ധു  | rokon        | хамаатан |
| M1 Parent's sibling's child                   | M0     | cousin   | cousin  | cugino  | GAP | GAP         | GAP     | GAP    | unokatestvér | үеэл     |
| M2 Parent's sibling's female child            | M1     | GAP      | cousine | cugina  | GAP | GAP         | GAP     | GAP    | GAP          | GAP      |
| M3 Elder daughter of mother's sibling         | M2     | GAP      | GAP     | GAP     | 表姐  | GAP         | GAP     | GAP    | GAP          | GAP      |
| M4 Daughter of mother's sister                | M2     | GAP      | GAP     | GAP     | GAP | नौसेरा बहिन | GAP     | GAP    | GAP          | GAP      |
| M5 Elder daughter of mother's sister          | M4     | GAP      | GAP     | GAP     | GAP | GAP         | அக்கா   | ചെട്ടി | GAP          | GAP      |

**Corpus development.** The corpus was manually assembled with the help of native speakers. The native speakers had above-average understanding about language and linguistics (they were computational linguists). They were presented with the set of 32 concepts, their definitions, and their lexicalizations in English. Contributors were encouraged to cross-check their input with traditional and online dictionaries, and the final choices were thoroughly discussed whenever the decision between lexicalization and gap was not straightforward (e.g. the Hungarian words *nagytestvér* and *kistestvér*, meaning *elder sibling* and *younger sibling*, resp., are informal and are used more rarely than the others). Let us note that the actual choice of words did not matter in the quantitative evaluation, only the indication of the presence or absence of it did. Still, the actual words are provided below for verification purposes.

On the basis of the lexicalization data, we produced 1,959 gold-standard interlingual equivalence, hypernymy, and untranslatability mapping relations. We generated all language-specific concepts (i.e. synsets) in the nine languages and computed all interlingual equivalence, hypernymy, and untranslatability relations. Equivalence exists between synsets lexicalized in two different languages (e.g. the English *sibling* and the Hungarian *testvér*). Hypernymy exists between a broader term in a language and a narrower term in another language (e.g. the English *sibling* and the Hungarian *öcs*, *younger brother*). In order to identify all instances of hypernymy, we relied on the hypernymy relations existing among the 32 language-independent concepts (e.g. *younger brother* is narrower than *sibling*). Finally, an untranslatability relation is defined between a lexicalization in a language and the absence of an equivalent in another language (e.g. the English *sibling* and its non-existent Italian equivalent). We did not include inverse relations into the dataset.

**Evaluation method.** We evaluated the theoretical coverage of the 1,959 gold-standard mappings by five state-of-the-art MLDBs, based on their mapping abilities. This meant producing  $5 \times 1959 = 9795$  binary data points indicating the presence or absence of support for each mapping. The data points were computed in a semi-automated manner, based on prior knowledge about the structure of each MLDB. For example, BabelNet does not represent lexical gaps, therefore all untranslatability relations were marked for absence of support. OMW supports the interlingual equivalence relation between two lexicalizations  $l_A$  and  $l_B$  in languages  $A$  and  $B$  iff  $\exists l_{\text{ENG}}$  such as  $l_A \equiv l_{\text{ENG}} \equiv l_B$ , that is, an equivalent English lexicalization exists; the same rule is applied to IndoWordNet but with the requirement of the existence of a Hindi lexicalization  $l_{\text{HIN}}$ .
